# Supplementary material for: New approach for the quantification of uncertainties in reaction modeling via data-driven multi-objective optimization
Source: arXiv:2507.06370 source file (2026-06-10)
Supplement: Supplementary file 1 [file Supplemental_material.pdf]

# Supplemental Material for "New approach for the quantification of uncertainties in reaction modeling via data-driven multi-objective optimization."

N. Dimitrakopoulos[1],* G. Perdikakis[1],† F. Montes[2], P. Gastis[3], S. A. Kuvin[3], H. Y. Lee[3], P. Tsintari[2], and A. V. Voinov[4]

[1] *Department of Physics, Central Michigan University, Mt. Pleasant, MI 48859, USA*
[2] *Facility for Rare Isotope Beams, Michigan State University, East Lansing, MI 48824, USA*
[3] *Los Alamos National Laboratory, Los Alamos, New Mexico 87545, USA and*
[4] *Department of Physics & Astronomy, Ohio University, Athens, OH 45701, USA*

This document provides additional technical information and supporting plots that complement the main article. It includes a description of the NSGA-II algorithm employed for the optimization, details on the implementation, and visualizations of the resulting parameter distributions and Pareto front projections.

## I. STRUCTURE OF THE NSGA-II OPTIMIZATION ALGORITHM

The optimization process starts by initializing a population of candidate solutions, which are then evaluated based on their objective values. The algorithm sorts the population into non-dominated fronts, where the first front consists of the best (non-dominated) solutions, and subsequent fronts contain solutions dominated only by those in earlier fronts. To maintain diversity, it computes a crowding distance for each solution, which measures its relative spacing in the objective space. Parent selection follows a binary tournament, prioritizing solutions with better Pareto rank and, in cases of ties, those with higher crowding distance. New solutions are generated using crossover and mutation operators, ensuring the exploration of the solution space. The offspring and parent populations are then merged, non-dominated sorting is reapplied, and the best solutions are retained for the next generation.

## II. PARAMETER EXPLORATION LIMITS

The search space for the OMP parameters was determined by systematically varying each parameter to extreme values and evaluating the $\chi^2_\nu$ for each reaction channel individually. The upper and lower bounds were determined by selecting parameter values that resulted in reduced chi-square values of approximately 20, which served as a practical cutoff for excluding clearly unphysical sets of parameters. The ranges for the OMP scaling parameters span from 0.75 to 1.25 and are detailed in Table I, along with the initial ranges of all parameters used to sample the first generation of solutions during the optimization process.

The spin cut-off parameter multiplier was varied between 0.5 and 2.0, while the values of the pre-equilibrium partial level density multiplier ($g$) that we explored ranged between 0.5 and 1.6.

For nuclei with available experimental data on their s-wave resonance spacings, the $a(S_n)$ parameter was varied within ±10% from the values reported in RIPL-3 ([1]). For all the other nuclei lacking experimental data we adopted a range of ±20% around the systematic value. This systematic value is calculated by substituting the $\tilde{a}$ value derived from systematics into ignatyuk formula :

$$a(S_n) = \tilde{a}(1 + \delta W(\frac{1 - e^{-\gamma(S_n - \Delta)}}{S_n - \Delta})) \qquad (1)$$

The formula for $\tilde{a}$, based on systematics, is expressed as:

$$\tilde{a} = d_1 A + d_2 A^{\frac{2}{3}} \qquad (2)$$

where $d_1, d_2$ are obtained from the global parametrization of Koning and Delaroche.

Finally, the ranges for the asymptotic parameter($\tilde{\alpha}$ can be obtained by solving eq. 1 for the damping parameter :

$$\gamma = -\frac{1}{S_n - \Delta} ln\left[1 - \frac{S_n - \Delta}{\delta W}\left(\frac{\alpha(S_n)}{\tilde{\alpha}} - 1\right)\right] \qquad (3)$$

under the constraint that the damping parameter needs to remain positive (effectively demanding the natural logarithm to be negative). Consequently, the upper and lower limits for the $\tilde{a}$ value are :

$$\frac{a_{min}(Sn)}{\frac{Sn-\Delta}{\delta W} + 1} < \tilde{a} < a_{max}(Sn) \qquad (4)$$

### A. Constraints

To restrict the parameter search space, we applied sets of inequality and equality constraints to penalize non-physical solutions. For example, the available experimental data for the s-wave resonance spacing ($D_0$) were utilized as constraints, requiring that our calculated $D_0$ values lie within the experimental uncertainty. In cases

* dimit2n@cmich.edu
† perdi1g@cmich.edu

TABLE I: Parameter ranges used in the optimization process. These bounds define the feasible search space for each parameter. The 200 solutions of first generation were randomly sampled within these ranges.

| Particle | Quantity | Talys keyword | Lower limit | Upper limit |
|---|---|---|---|---|
| proton | $(r_V)$ | rvadjust p | 0.750 | 1.259 |
| | $(a_V)$ | avadjust p | | |
| alpha | $(r_V)$ | rvadjust $\alpha$ | 0.950 | 1.050 |
| | $(a_V)$ | avadjust $\alpha$ | | |
| neutron | $(r_V)$ | rvadjust n | 0.750 | 1.200 |
| | $(a_V)$ | avadjust n | | |
| $^{65}Ni$ | $a(Sn)$ | a 28 65 | 8.942 | 10.930 |
| | $\tilde{a}$ | alimit 28 65 | 7.060 | |
| $^{64}Cu$ | $a(Sn)$ | a 28 64 | 7.63 | 9.325 |
| | $\tilde{a}$ | alimit 28 64 | 7.63 | 9.639 |
| $^{65}Cu$ | $a(Sn)$ | a 28 65 | 7.524 | 11.287 |
| | $\tilde{a}$ | alimit 28 65 | 7.089 | |
| $^{67}Cu$ | $a(Sn)$ | a 28 65 | 8.245 | 12.367 |
| | $\tilde{a}$ | alimit 28 65 | 6.912 | |
| $^{68}Cu$ | $a(Sn)$ | a 28 68 | 8.533 | 12.800 |
| | $\tilde{a}$ | alimit 28 68 | 6.715 | |
| $^{66}Zn$ | $a(Sn)$ | a 30 66 | 7.771 | 11.656 |
| | $\tilde{a}$ | alimit 30 66 | 7.075 | |
| $^{67}Zn$ | $a(Sn)$ | a 30 67 | 9.673 | 11.823 |
| | $\tilde{a}$ | alimit 30 67 | 7.270 | |
| $^{68}Zn$ | $a(Sn)$ | a 30 68 | 8.954 | 10.943 |
| | $\tilde{a}$ | alimit 30 68 | 7.061 | |
| $^{69}Zn$ | $a(Sn)$ | a 30 69 | 10.350 | 12.650 |
| | $\tilde{a}$ | alimit 30 69 | 6.788 | |
| $^{66}Ga$ | $a(Sn)$ | a 31 66 | 7.530 | 11.295 |
| | $\tilde{a}$ | alimit 31 66 | 7.248 | |
| $^{67}Ga$ | $a(Sn)$ | a 31 67 | 7.980 | 11.970 |
| | $\tilde{a}$ | alimit 31 67 | 7.180 | |
| | $g$ | gadjust 31 68 | 0.600 | 1.600 |
| $^{68}Ga$ | $a(Sn)$ | a 31 68 | 8.369 | 12.553 |
| | $\tilde{a}$ | alimit 31 68 | 7.039 | |
| | $g$ | gadjust 31 68 | 0.600 | 1.600 |
| $^{69}Ga$ | $a(Sn)$ | a 31 69 | 8.769 | 13.154 |
| | $\tilde{a}$ | alimit 28 65 | 7.038 | |
| | $g$ | gadjust 31 68 | 0.600 | 1.600 |
| $^{70}Ge$ | $a(Sn)$ | a 32 70 | 8.904 | 13.356 |
| | $\tilde{a}$ | alimit 32 70 | 7.086 | |
| $^{71}Ge$ | $a(Sn)$ | a 32 71 | 11.81 | 14.434 |
| | $\tilde{a}$ | alimit 32 71 | 7.682 | |
| Global | $\sigma$ | Rspincut | 0.500 | 2.000 |

where the difference exceeded the experimental uncertainty, an exponential penalty function was applied, ensuring that larger deviations resulted in stronger penalties.

We imposed additional constraints on the parameter space to prevent recalculations of the shell correction value for all nuclei involved, which would otherwise be required when physically inconsistent parameter combinations lead to negative damping parameters. These constraints stem from Eq. 3, as we are working within a defined range for $a(Sn)$ and $\tilde{a}$. If $\tilde{a}$ is chosen near its upper limit, while $a(\mathrm{Sn})$ is selected at the lower edge of the allowed range, there is a risk that the damping parameter becomes negative. To exclude such combinations of parameters from the search space, a penalty factor of 1e6 was applied whenever the optimization process resulted in negative damping parameters.

The remaining 18 constraints required that the $\chi^2_\nu$ values between experimental and calculated data be lower than those obtained using the global parametrization. However, we only penalized solutions if their $\chi^2_\nu$ exceeded the default value by more than 2.5. This more lenient approach was necessary because our $\chi^2_\nu$ calculation only accounted for statistical uncertainties, as systematic uncertainties were not consistently provided across the datasets. Furthermore, for cases where x-axis uncertainties were missing and no indication was given to estimate them, we assigned a minimum uncertainty of 5 keV. These considerations ensured a fairer comparison between different datasets while preventing the overpenalization of solutions due to incomplete uncertainty information. If a solution exceeded this 2.5 limit, a penalty was applied proportionally to the fraction of the cross-section for the specific reaction channel relative to the total cross-section. For example, deviations in reaction channels with cross-sections around 1 barn were penalized by multiplying their difference by 1000, while for cross-sections below 1 mb, the penalty was simply the reduced chi-square value without any additional multiplier.

## III. PARAMETER DISTRIBUTIONS

In Fig. 1, we present the resulting distributions for the optimized parameters used in this work. The global values for these parameters used by TALYS code are also shown for comparison, along with the kernel density estimator (KDE) of each of the parameter distributions.

Many parameters exhibit bimodal distributions, reflecting the interplay between the strict definition of Pareto optimality and the constraints imposed in this work. To approximate the resulting uncertainty bands, without supplying the full set of Pareto-optimal solutions, we adopted a simplified approach based on random sampling

For each parameter, we identified the most probable value from its KDE and selected a sampling range around it. These ranges were chosen so that uniform random sampling within them produces cross-section uncertainty bands comparable to those obtained from the full Pareto-optimal set. Specifically, the width of each uncertainty band was defined as the envelope between the maximum and minimum predicted cross sections at each energy point. The sampling ranges were adjusted so that the simplified bands differed by no more than 20 percent from the Pareto-derived bands in any reaction channel.

This simplified sampling approach does not capture parameter correlations and therefore tends to slightly overestimate uncertainties in some reaction channels. The full Pareto set, in contrast, reflects compensating corre-

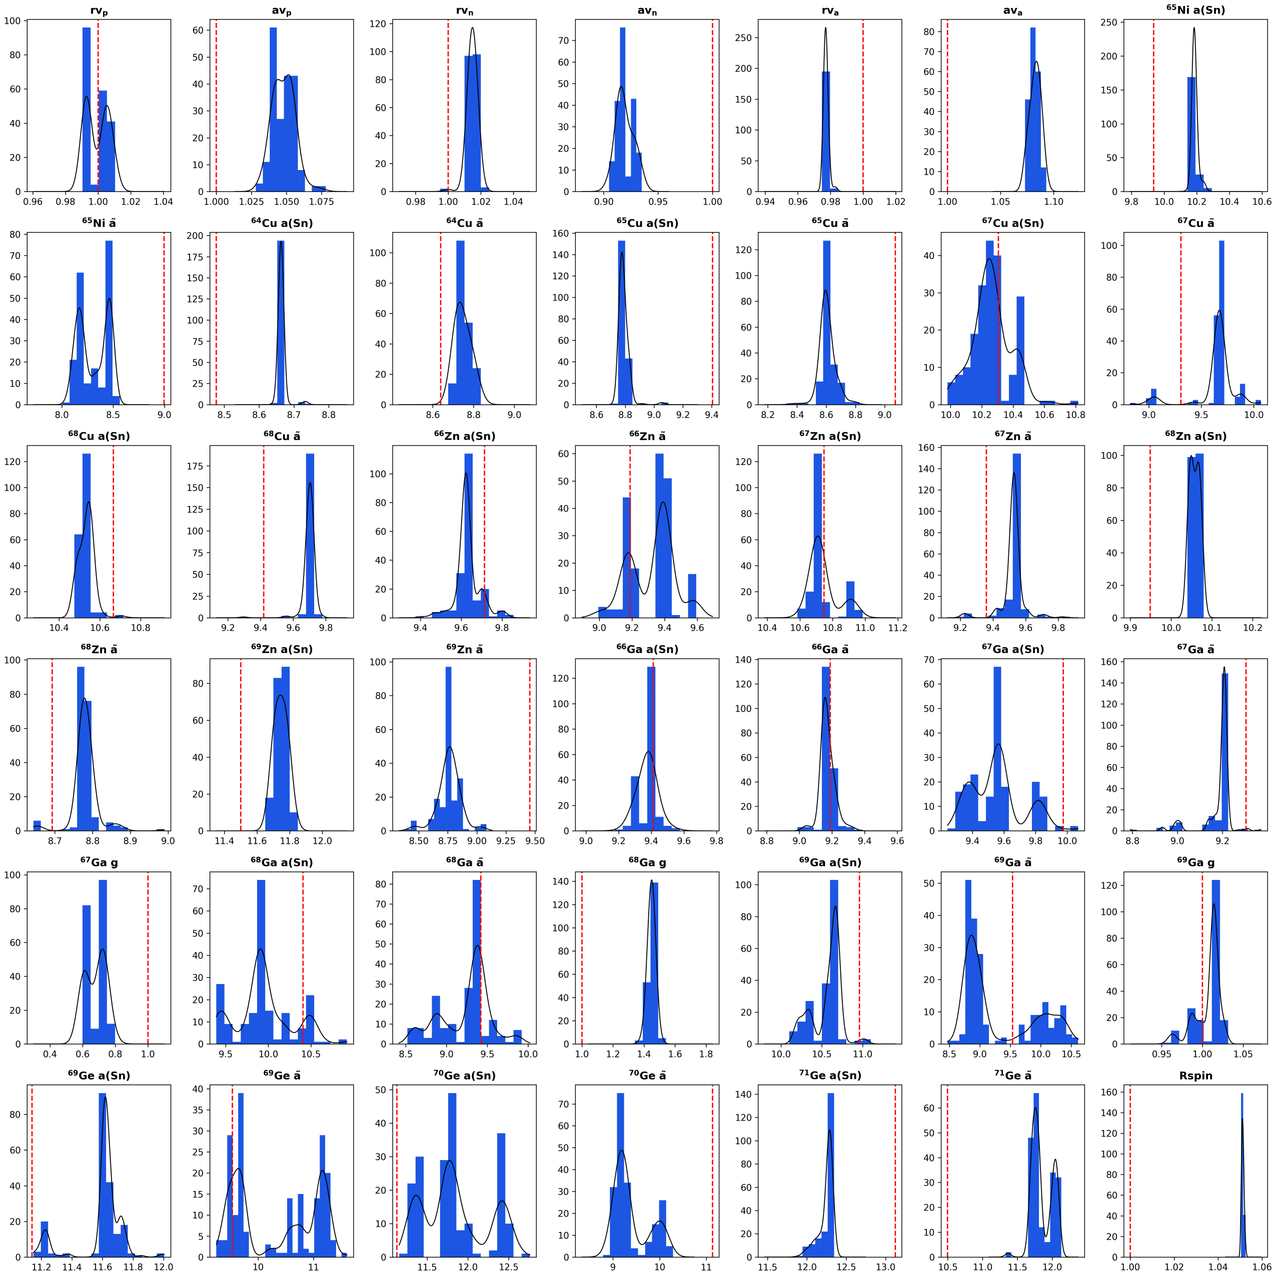


FIG. 1: Resulting distributions for all the parameters optimized in this work.The dashed red lines represent the global values used in TALYS 2.0. The solid green line shows the kernel density estimate (KDE), providing a smoothed representation of the underlying distribution for each parameter.

lations among parameters, which can reduce the spread of predicted cross sections even in the presence of individual parameter extremes.

The full set of 200 Pareto-optimal parameter combinations is provided in the supplementary material, allowing for exact reproduction of the original uncertainty bands.

To further assess parameter interdependence, we used the distance correlation method [2], with results shown in Fig. 2. Most parameter pairs exhibited correlations below 0.3, with a maximum value of 0.58. This generally weak correlation supports the use of random sampling, as strong dependencies are not prevalent. Distance correlation was chosen because it captures both linear and nonlinear relationships, providing a more general measurement of statistical dependence. For comparison, Spearman correlation coefficients were also computed and found to be small, typically ranging between -0.15 and 0.15.

To quantify these distributions, Table II provides various statistical measures for each parameter. The mini-

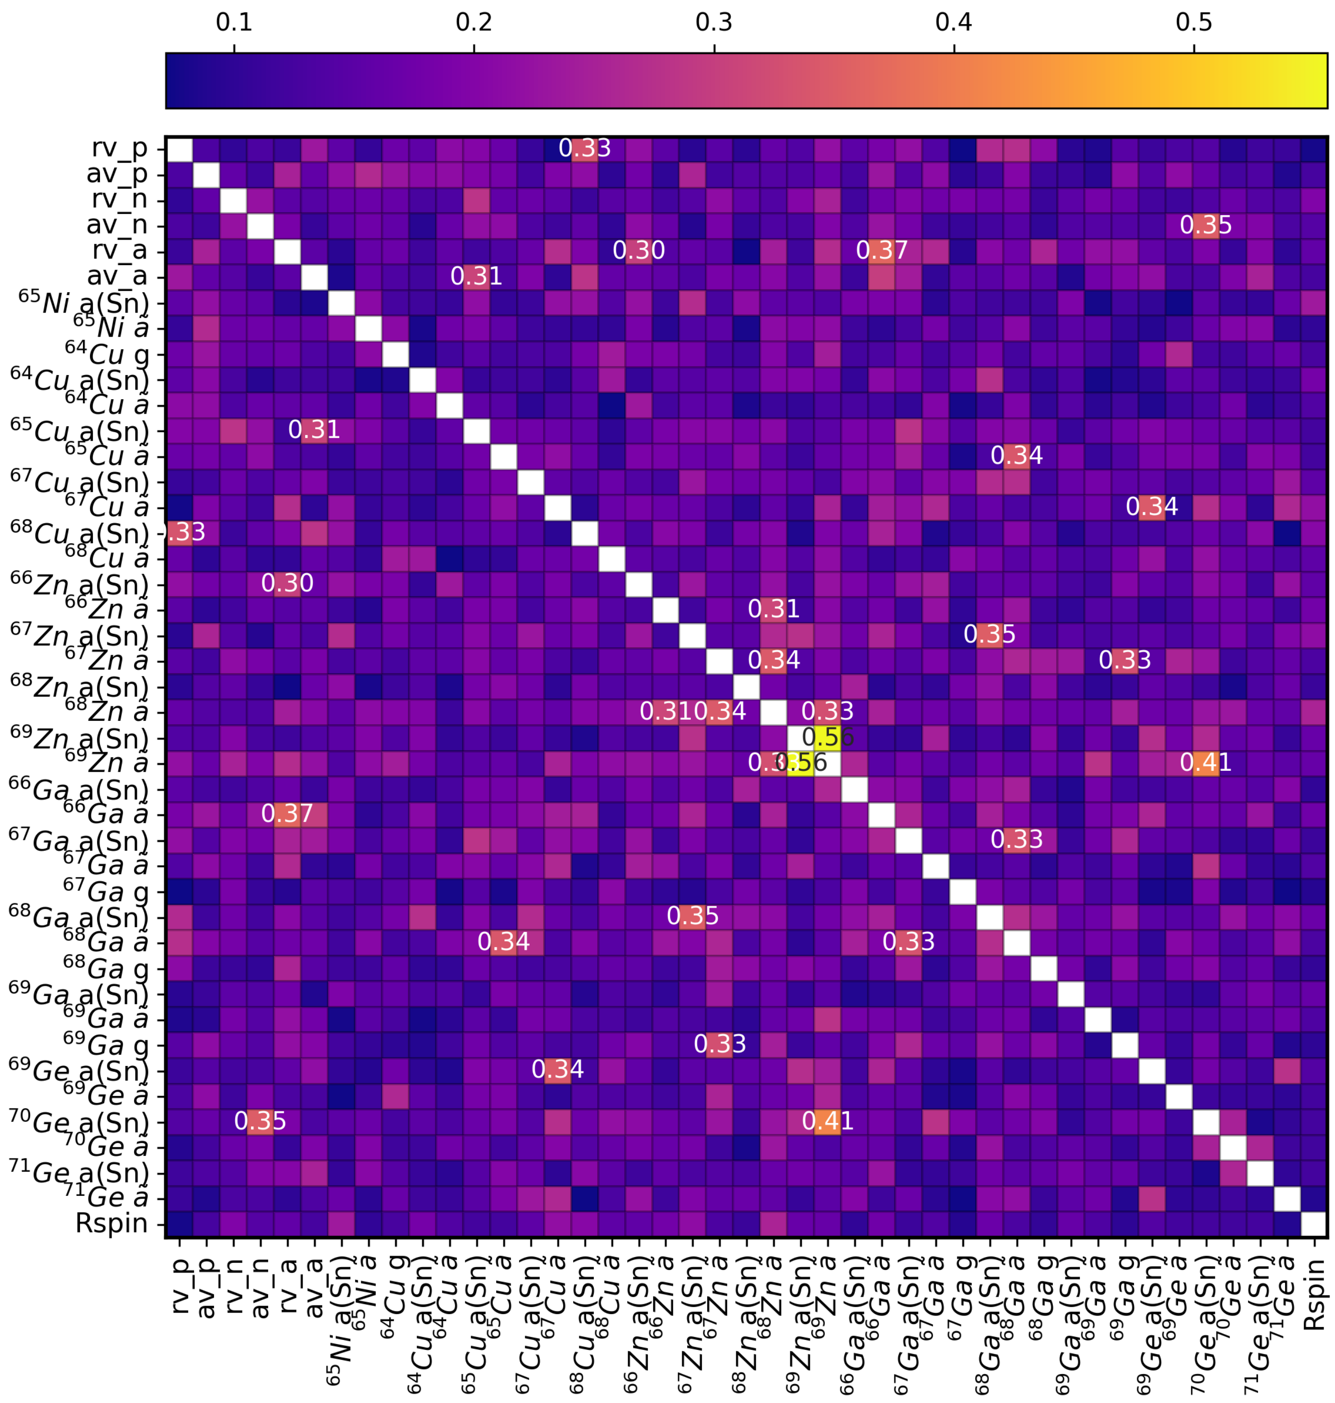


FIG. 2: Distance correlation matrix for the 42 parameters used in this work. The distance correlation method captures both linear and nonlinear associations between parameters. Overall, only weak correlations are observed. Correlation values above 0.30 are annotated for reference.

mum and maximum values allow for a direct comparison with the initial parameter ranges used during optimization (Table I ). Additionally, the mean, standard deviation, and interquartile range (IQR) are presented. The IQR measures the spread of the middle 50% of the data. Given the multimodal nature of the distributions, we employed the bootstrap resampling technique [3] to further investigate the variability and potential biases in the optimized parameters. Bootstrapping generates multiple resampled datasets by drawing randomly with replacement from the original data. In this study, we performed 50 bootstrap resamplings. We computed the 97% confi-

dence intervals for the median values using the bootstrap approach. To complement this, we determined the Kernel Density Estimation (KDE) peak, which identifies the most probable value within each parameter's distribution.

## IV. BENCHMARK

To further validate our method, we calculated the cross sections for the $^{66}$Zn$(\alpha, n)^{69}$Ge and $^{64}$Zn$(\alpha, np)^{67}$Ga reactions (Fig. 3), which were not included in the original optimization process.

For both $^{64}$Zn and $^{66}$Zn, the TALYS-recommended optical model parameters (OMPs) were used, as well as the default pre-equilibrium density parameter $g$ for their respective residual nuclei. However, the nuclear level density (NLD) parameters were taken from the results of our optimization, applied to residual nuclei involved in the corresponding and competing $(\alpha, x)$ reaction channels.

In the case of the $^{66}$Zn$(\alpha, n)^{69}$Ge reaction, the NLD parameters used for both the compound nucleus and the residual nucleus ($^{69}$Ge) were those optimized in this work. Additionally, the NLD parameters for $^{69}$Ga—relevant to the competing $(\alpha, p)$ channel—were also optimized. For the $^{64}$Zn$(\alpha, np)^{67}$Ga reaction, which serves as the second benchmark case, only the residual nucleus $^{67}$Ga was part of the original optimization.

The uncertainty band in Fig.3, was determined by running TALYS with all the Pareto-optimal NLD parameters for every relevant nucleus of Table II. Our approach provides an uncertainty-quantified cross-section that is mostly in fair agreement with the existing data. The uncertainty band reflects the propagated uncertainty from the optimized NLD parameters to the cross-section of the "unknown" reaction. Further tuning of the optical potential could significantly improve the agreement at the low-energy part of the cross section. With this result, we show that with our approach, we can provide realistic estimates of cross-sections and address the community-identified need for realistic uncertainties consistent between model parameters and the resulting calculated cross-sections.

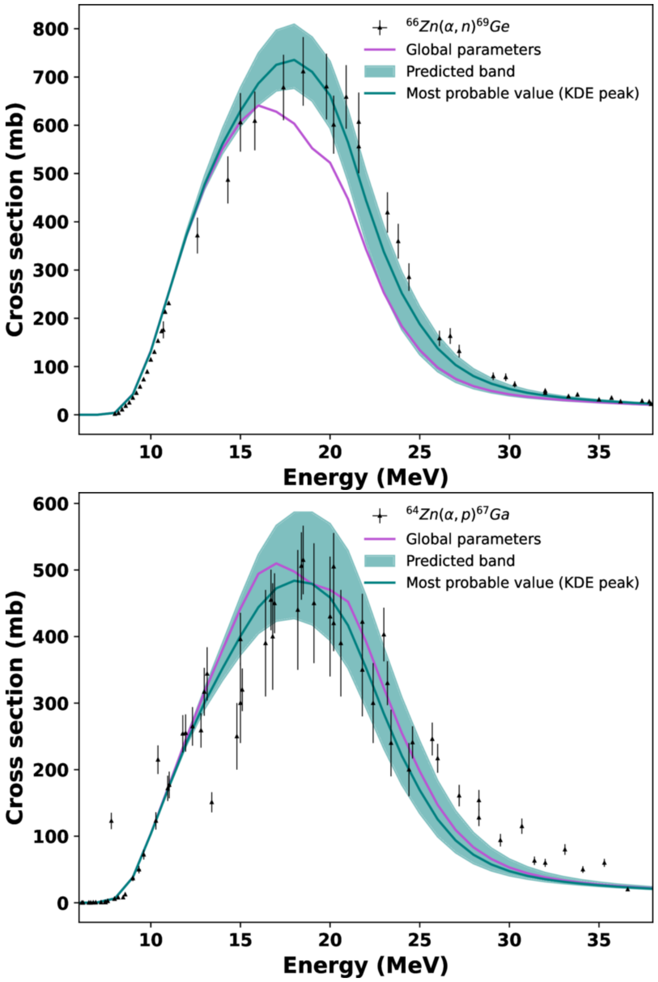


FIG. 3: Top: Predicted cross section for the $^{66}$Zn$(\alpha, n)^{69}$Ge reaction. Bottom: Predicted cross section for the $^{64}$Zn$(\alpha, p)^{67}$Ga reaction. Neither reaction was included in the optimization process. The teal band represents the uncertainty arising from the optimized NLD inputs relevant to each reaction. The teal line indicates the most probable prediction and is compared to the TALYS default calculation for both reactions.

TABLE II: Statistical measures for all optimized parameters, including the minimum and maximum values, mean, standard deviation (Std), interquartile range (IQR), kernel density estimate (KDE) peak, 95% confidence interval (CI) for the KDE peak obtained through bootstrap resampling with 50 resamples, and the full width at half maximum (FWHM) CI of the KDE. The table also compares these values to the default TALYS parameters.

| Parameter | [Min,Max] | Mean | Std | IQR | KDE Peak | KDE Peak CI | KDE FWHM CI | Default TALYS |
|---|---|---|---|---|---|---|---|---|
| $rv_\alpha$ | [0.976, 0.983] | 0.977 | 0.001 | 0.977 | [0.977, 0.977] | 0.977 | [0.977, 0.977] | 1.0 |
| $av_\alpha$ | [1.074, 1.092] | 1.083 | 0.005 | 1.083 | [1.082, 1.083] | 1.083 | [1.082, 1.087] | 1.0 |
| $rv_p$ | [0.99, 1.01] | 0.999 | 0.007 | 1.002 | [0.994, 1.004] | 0.996 | [0.993, 1.005] | 1.0 |
| $av_p$ | [1.032, 1.074] | 1.048 | 0.007 | 1.047 | [1.043, 1.051] | 1.047 | [1.042, 1.053] | 1.0 |
| $rv_n$ | [1.0, 1.02] | 1.015 | 0.002 | 1.015 | [1.014, 1.015] | 1.014 | [1.013, 1.017] | 1.0 |
| $av_n$ | [0.905, 0.935] | 0.919 | 0.007 | 0.917 | [0.916, 0.917] | 0.916 | [0.916, 0.916] | 1.0 |
| $^{65}$Ni a(sn) | [10.141, 10.244] | 10.188 | 0.014 | 10.183 | [10.183, 10.184] | 10.183 | [10.183, 10.184] | 9.936 |
| $^{65}$Ni $\tilde{a}$ | [8.071, 8.499] | 8.31 | 0.143 | 8.322 | [8.221, 8.377] | 8.362 | [8.164, 8.465] | 8.997 |
| $^{64}$Cu a(sn) | [8.647, 8.737] | 8.664 | 0.01 | 8.664 | [8.663, 8.664] | 8.663 | [8.663, 8.663] | 8.477 |
| $^{64}$Cu $\tilde{a}$ | [8.69, 8.82] | 8.747 | 0.033 | 8.728 | [8.727, 8.73] | 8.724 | [8.723, 8.724 | 8.639 |
| $^{65}$Cu a(sn) | [8.744, 9.055] | 8.789 | 0.035 | 8.782 | [8.778, 8.782] | 8.775 | [8.773, 8.777] | 9.405 |
| $^{65}$Cu $\tilde{a}$ | [8.367, 8.791] | 8.607 | 0.05 | 8.596 | [8.594, 8.596] | 8.592 | [8.59, 8.594] | 9.072 |
| $^{67}$Cu a(sn) | [9.981, 10.815] | 10.26 | 0.124 | 10.246 | [10.233, 10.262] | 10.247 | [10.239, 10.261] | 10.306 |
| $^{67}$Cu $\tilde{a}$ | [8.823, 10.067] | 9.642 | 0.194 | 9.677 | [9.675, 9.677] | 9.672 | [9.669, 9.675] | 9.305 |
| $^{68}$Cu a(sn) | [10.485, 10.706] | 10.533 | 0.034 | 10.545 | [10.545, 10.545] | 10.548 | [10.547, 10.548] | 10.666 |
| $^{68}$Cu $\tilde{a}$ | [9.296, 9.763] | 9.699 | 0.036 | 9.709 | [9.708, 9.709] | 9.707 | [9.704, 9.71] | 9.420 |
| $^{66}$Zn a(sn) | [9.411, 9.821] | 9.632 | 0.058 | 9.625 | [9.624, 9.627] | 9.623 | [9.621, 9.624] | 9.714 |
| $^{66}$Zn $\tilde{a}$ | [8.996, 9.591] | 9.324 | 0.135 | 9.38 | [9.368, 9.385] | 9.39 | [9.388, 9.393] | 9.189 |
| $^{67}$Zn a(sn) | [10.621, 10.947] | 10.743 | 0.083 | 10.713 | [10.711, 10.718] | 10.711 | [10.709, 10.714] | 10.748 |
| $^{67}$Zn $\tilde{a}$ | [9.217, 9.825] | 9.523 | 0.065 | 9.528 | [9.528, 9.528] | 9.528 | [9.527, 9.53] | 9.359 |
| $^{68}$Zn a(sn) | [10.045, 10.075] | 10.058 | 0.011 | 10.063 | [10.048, 10.065] | 10.048 | [10.047, 10.064] | 9.949 |
| $^{68}$Zn $\tilde{a}$ | [8.644, 8.99] | 8.781 | 0.034 | 8.778 | [8.775, 8.78] | 8.778 | [8.776, 8.779] | 8.693 |
| $^{69}$Zn a(sn) | [11.687, 11.815] | 11.746 | 0.035 | 11.725 | [11.722, 11.771] | 11.745 | [11.715, 11.776] | 11.5 |
| $^{69}$Zn $\tilde{a}$ | [8.427, 9.036] | 8.762 | 0.093 | 8.762 | [8.76, 8.766] | 8.765 | [8.762, 8.768] | 9.454 |
| $^{66}$Ga a(sn) | [9.193, 9.557] | 9.374 | 0.052 | 9.384 | [9.383, 9.386] | 9.387 | [9.386, 9.388] | 9.413 |
| $^{66}$Ga $\tilde{a}$ | [9.034, 9.341] | 9.172 | 0.042 | 9.158 | [9.157, 9.159] | 9.155 | [9.154, 9.156] | 9.189 |
| $^{67}$Ga a(sn) | [9.242, 10.069] | 9.556 | 0.165 | 9.563 | [9.547, 9.571] | 9.563 | [9.558, 9.567] | 9.975 |
| $^{67}$Ga $\tilde{a}$ | [8.791, 9.371] | 9.184 | 0.07 | 9.206 | [9.205, 9.208] | 9.207 | [9.206, 9.208] | 9.305 |
| $^{67}$Ga g | [0.601, 0.798] | 0.678 | 0.059 | 0.71 | [0.698, 0.712] | 0.7 | [0.609, 0.724] | 1.0 |
| $^{68}$Ga a(sn) | [9.391, 10.921] | 9.948 | 0.33 | 9.922 | [9.902, 9.923] | 9.911 | [9.895, 9.924] | 10.407 |
| $^{68}$Ga $\tilde{a}$ | [8.56, 9.878] | 9.244 | 0.305 | 9.362 | [9.307, 9.379] | 9.378 | [9.368, 9.389] | 9.420 |
| $^{68}$Ga g | [1.386, 1.497] | 1.448 | 0.016 | 1.453 | [1.453, 1.453] | 1.453 | [1.453, 1.454] | 1.0 |
| $^{69}$Ga a(sn) | [10.166, 11.034] | 10.566 | 0.177 | 10.66 | [10.653, 10.668] | 10.662 | [10.656, 10.667] | 10.961 |
| $^{69}$Ga $\tilde{a}$ | [8.469, 10.611] | 9.308 | 0.607 | 8.98 | [8.891, 9.029] | 8.879 | [8.863, 8.898] | 9.536 |
| $^{69}$Ga g | [0.956, 1.027] | 1.007 | 0.015 | 1.013 | [1.013, 1.014] | 1.014 | [1.014, 1.014] | 1.0 |
| $^{69}$Ge a(sn) | [11.149, 12.003] | 11.59 | 0.157 | 11.617 | [11.615, 11.619] | 11.629 | [11.624, 11.634] | 11.139 |
| $^{69}$Ge $\tilde{a}$ | [9.246, 11.603] | 10.335 | 0.735 | 10.524 | [9.758, 10.585] | 9.896 | [9.567, 11.124] | 9.536 |
| $^{70}$Ge a(sn) | [11.251, 12.663] | 11.847 | 0.393 | 11.787 | [11.771, 11.807] | 11.781 | [11.768, 11.794] | 11.130 |
| $^{70}$Ge $\tilde{a}$ | [8.894, 10.181] | 9.397 | 0.372 | 9.233 | [9.226, 9.239] | 9.194 | [9.177, 9.205] | 9.651 |
| $^{71}$Ge a(sn) | [11.892, 12.317] | 12.245 | 0.086 | 12.288 | [12.286, 12.289] | 12.289 | [12.288, 12.291] | 13.122 |
| $^{71}$Ge $\tilde{a}$ | [11.366, 12.097] | 11.854 | 0.147 | 11.801 | [11.789, 11.804] | 11.758 | [11.746, 11.772] | 10.496 |
| Rspin | [1.051, 1.052] | 1.051 | 0.0 | 1.051 | [1.051, 1.051] | 1.051 | [1.051, 1.051] | 1.0 |

[1] R. Capote, M. Herman, P. Obložinský, P. Young, S. Goriely, T. Belgya, A. Ignatyuk, A. Koning, S. Hilaire, V. Plujko, M. Avrigeanu, O. Bersillon, M. Chadwick, T. Fukahori, Z. Ge, Y. Han, S. Kailas, J. Kopecky, V. Maslov, G. Reffo, M. Sin, E. Soukhovitskii, and P. Talou, Ripl – reference input parameter library for calculation of nuclear reactions and nuclear data evaluations, Nuclear Data Sheets **110**, 3107 (2009), special Issue on Nuclear Reaction Data.

[2] G. J. Székely and M. L. Rizzo, Brownian distance covariance, The Annals of Applied Statistics **3**, 1236 (2009).

[3] B. Efron, Bootstrap Methods: Another Look at the Jackknife, The Annals of Statistics **7**, 1 (1979).
